# Supplementary material for: A Comparison of Self-Play Algorithms Under a Generalized Framework
Source: arXiv:2006.04471 source file (2020-06-08)
Supplement: Supplementary file 1 [file appendix.tex]

\documentclass{../main.tex}{}

\begin{document}

\end{document}
